# Supplementary material for: PG-Schema: Schemas for Property Graphs
Source: arXiv:2211.10962 source file (2023-07-08)
Supplement: Supplementary file 1 [file 7-appendix.tex]

\section{A Graph-based Data Catalog}

%\begin{example}[A Graph-based Data Catalog]\label{ex:1}

An enterprise data catalog is a  metadata management tool that companies use to inventory data resources and organize the data within their systems. Data catalogs enable data discovery in order to empower the company’s workforce to search and find data, get more information from data investments, gaining better data insights as a whole, and making smart business decisions quickly.

To accomplish this, data catalogs need to create and manage collections of data and curate the relationships among them, to provide a unified view of the data landscape to data producers (e.g. data engineers) and data consumers (e.g. data scientists and analysts).  These collections traditionally include tables and columns of a database, business glossary terms, analysis, and reports from BI dashboards, but quickly evolve to include all types of data resources  (e.g. ETL tools, DBT models, proprietary data systems, ML models, the latest data tech, etc).

Businesses evolve quickly, and with that evolution come changes in the data landscape. For example, when a company acquires another company, they also acquire all their data systems. These new data systems need to be catalogued and related to the existing business terminology, in order to provide a holistic view of the new data landscape. Thus, a data catalog must be able to keep up with the pace of business evolution, and understand what data resources exist, what new data resources are coming in, and how these are related. Therefore, there is a need to have a formalism to describe the set of known data resources and the growing and evolving set of unknown data resources that a company may encounter. This evolution can be empowered by \pgschema{} (R7), allowing for flexible definitions of node types, content types and relationship types. 

Property Graphs provide an intuitive way to model data catalog concepts via different kinds of relationships. The catalogs and different types of data resources the contain (such as databases tables, columns, or any other data injected in the system) are naturally modelled as graph nodes; the containment relationships are encoded as typing inheritance relationships (R6) (i.e. tables, columns etc. are node subtypes of the resource node type), while the data lineage relationships (such as the information about derivations of each resource from other resources) can be represented as graph edges. Exploring a dataset and its downstream resources can be easily represented as quantified path pattern matching \cite{DeutschFGHLLLMM22}. Furthermore, as new data resources emerge and their attributes evolve, schema needs to accommodate the changes flexibly (R7). 
%Property Graphs provide an intuitive way to model data catalog concepts via different kinds of relationships: catalogs and different types of data resources (such as databases tables, columns and any other data resource injected in the system) they contain are naturally modelled as graph nodes; the containment relationships are encoded as typing inheritance relationships (R6) (i.e. tables, columns etc. are node subtypes of the resource node type) while the data lineage relationships (such as the information about derivations of each resource from other resources) can be represented as graph edges between nodes. Exploring a dataset and its downstream resources can be easily represented as quantified path pattern matching \cite{DeutschFGHLLLMM22}. Furthermore, as new data resources emerge and their attributes evolve, schema needs to accommodate the changes flexibly (R7). 

Property Graph schemas need to capture node and edge types, type hierarchy, meanwhile providing flexibility for a fast-evolving business landscape where new data types and relationships emerge frequently. For example, if a schema is defined for a certain type (e.g. Data Transformation resource), and a new subtype is defined representing a new data resource that has been acquired (e.g. Vendor A’s  ETL tool resource), the data catalog’s integrity needs to be enforced based on the original type (R6) . Combinations of flexible schemas with partial schemas can be devised in this case, to cover the evolution of data catalogs.
%(as illustrated in Table\ref{tab:quadrants})

Figure \ref{fig-uc1} illustrates the \pgschema{} of a data catalog. Node types (R1) include \inlinecode{Catalog} representing the collection of data resources, the abstract type \inlinecode{DataResource} representing all data resources, and its subclasses (R6) \inlinecode{Database}, \inlinecode{Table}, \inlinecode{Column} etc. each representing a concrete data resource type. Edge types (R2) include \inlinecode{hasResource} connecting \inlinecode{Catalog} nodes to any \inlinecode{DataResources} nodes, \inlinecode{derivedFrom} connecting \inlinecode{DataResources} to \inlinecode{DataResources} indicating their lineage, and other types such as \inlinecode{hasTable} and \inlinecode{hasColumn} indicating the containment relationships between data resources. Node and edge types have also defined their properties (R3). Some of the specified types (\inlinecode{CatalogGraph}, \inlinecode{Table}, \inlinecode{Column} etc.) have identities (R4). 

\begin{figure}[t!]
\begin{lstlisting}
CREATE GRAPH TYPE CatalogGraphType STRICT {
  (CatalogType: Catalog {id INT}),
  (DataResourceType: DataResource),
  (DatabaseType: DataResourceType
    {path STRING, owner STRING}),
  (TableType: DataResourceType {id INT, name STRING}),
  (ColumnType: DataResourceType
    {id INT, name STRING, dataType STRING}),
  (GraphType: DataResourceType {id INT, name STRING}),
  (:CatalogType)
    -[HasResourceType: hasResource {since DATE}]->
  (:DataResourceType),
  (:DataResourceType)
    -[DerivedFromType: derivedFrom {since DATE}]->
  (:DataResourceType),
  (:DatabaseType)-[HasTableType: hasTable {since DATE}]->
  (:TableType),
  (:TableType)-[HasColumnType: hasColumn {since DATE}]->
  (:ColumnType),
  FOR (CatalogType) EXCLUSIVE c.id WITHIN (c CatalogType)
  ...
}
\end{lstlisting}
\caption{\pgschema{} of a graph-based data catalog.}
\label{fig-uc1}
\end{figure}

\pgschema{}  are by definition flexible and agile, and by building a data catalog on a property graph and its companion \pgschema{}, they enable the flexibility of extending that same graph schema across any new sources of data that organizations acquire (R7--R8). Schema validation and efficient error reporting (R11) must be guaranteed thanks to the 
agile property types and constraints. In fact, the very nature of a property graph schema makes it easy to extend the data catalog alongside growing graph ecosystems \cite{SakrBVIAAAABBDV21}.

\section{Existing Graph Schema Languages}

\paragraph{Conceptual Data Models} 

By \emph{conceptual data models} we mean here data models that aim to be conceptual in nature, 
i.e., closer and more faithful to 
the \emph{Universe of Discourse} of the stakeholders than 
traditional database models, such as the relational model,
aim to be. 
Typical examples of conceptual data models are 
the Entity-Relationship Model \cite{Chen1976} and its various extensions which are usually described as EER models
and include  
the \emph{Extended Entity-Relationship Model} \cite{Thalheim_extended_2018}
and the various \emph{Enhanced Entity-Relationship Models} that can be found
in database textbooks such as \cite{Elmasri_fundamentals_2015}.
Other conceptual data models that were inspired by ER but have some important differences are
\emph{ORM2 diagrams} \cite{halpin2015} and
\emph{UML Class diagrams} when used for the conceptual perspective \cite{Fowler2003}. 

Typically conceptual data models are not used as native data models of DBMSs or data stores, but are mapped to the data model that is supported by the DBMS that is used in the implementation.
Therefore the semantics of diagrams in ER, EER, and ORM are usually defined in terms of mappings to the relational model.
They have in common that the data is modelled in terms of entities, relationships and attributes, although there is variation in how these are exactly defined.
The ability to express constraints is typically limited to what can be effectively mapped to an SQL DBMS, with the notable exception of UML Class diagrams which allow constraints to be expressed in the Turing-complete language OCL.

% \textcolor{purple}{TO DISCUSS:
% \begin{description}
%     \item[In common:] \pgschema leans towards conceptual (but prefers easy-to-implement over being conceptually faithful)
%     \item[Difference:] \pgschema is not restricted to schema-first (so there is a notion if instance that is independent from a schema) but intends to cover the whole spectrum from schema-first to schema-last.
%    \item[Difference:] Separation between \emph{labels} and \emph{types}.
%    \item[Difference:] \pgschema is part of query language formalism (so typing is closer in philosophy to programming-language typing)
%    \item[Difference:] \pgschema anticipates partial typing (not all parts of the graph are restricted by the schema) and open typing (in some places types can be partially open and allow any kind of value)    
%\end{description}
%}

\paragraph{RDF formalisms} The Resource Description Framework (RDF) \cite{Lanthaler2014RCA} is the World Wide Web Consortium (W3C) recommendation for representing data interchange on the Semantic Web \cite{Berners2001semantic}. 
RDF corresponds to a directed, edge-labeled multigraph, which links Web resources. These are identified by Internationalized Resource Identifiers (IRIs) and described by properties and property values. 
Thus, an RDF graph is a set of triples, each specifying a given resource’s identifier (subject node), property (predicate edge), and corresponding property value (object node). 
RDF is innately self-describing and prominently supports a \emph{schema-flexible approach}%\hannes{The introduction calls this \emph{flexible schema}. 
%The term used here should be aligned. 
%I also do not see schema-last being introduced as a term anywhere. It is also a confusing term, because schema in schema formation is present even if no schema is enforced. 
%The data is not without a schema at any time. If it would you would not able to query it. The simplest would be to use \emph{flexible schema} here, like in the intro.} 
whereby data is allowed to evolve naturally, unconstrained by an a priori schema. 
To describe the structure of RDF data, the W3C proposed the RDF Schema (RDFS) \cite{Brickley2014RS} and, subsequently, the Web Ontology Language (OWL) \cite{Hitzler2012OWO}. 
Both provide additional vernacular for resource properties and classes and, thus, allow the organizing of RDF data according to a typed hierarchy. 
Recently, RDF data shape languages \cite{Tomaszuk2017rdf} (e.g. SHACL \cite{Knublauch2017SCL,CormanRS18}, ShEx \cite{Baker2019,Staworko2015complexity}, ReSh \cite{ryman2013oslc}) have been proposed to address the growing need for schemas for RDF and describing RDF graph structures. 
It should be mentioned that RDF Schema, contrary to what its name may suggest, is not a schema language in the classical sense but is primarily used to infer implicit facts. 
RDF data shape languages define conditions that RDF (data) graphs must meet to be considered "conformant": which nodes and edges may appear in a given graph, in what combinations, and with what datatypes. 
The main difference between RDF formalisms and our proposal is that RDF does not support properties for edges\footnote{RDF-star supports this feature, but currently, solutions such as SHACL and ShEx do not support RDF-star \cite{Hartig2017rdf}}. Both ShEx and SHACL allow greater expression possibilities in the areas of cardinality, constraints on values, and datatype facets.

\paragraph{Tree-structured data} Tree-structured data is organized in a hierarchy that starts from a root element and branches out to its child elements, each of which can have further sub-elements. Prominent tree-structured data languages include XML and JSON, each with their dedicated schema formalisms.

For XML, the main schema languages are Document Type Definition (DTD) \cite{Yergeau2008EML}, XML Schema \cite{SperbergMcQueen2012WXS}, and REgular LAnguage for XML Next Generation (RELAX NG) \cite{ISO19757-2}. The former specifies, for each element: 1) a regular expression defining the permitted names of its child nodes, 2) a list of associated attribute names and whether they are mandatory, and 3) a description of textual content of elements and attributes. Note that, in DTD,  there is no distinction between element names and their types. This is supported by XML Schema and RELAX NG. These allow complex type definitions for child nodes and the usage of  simple types (strings, dates, integers, etc.) to describe the content pattern of elements and attributes.

JSON Schema \cite{Wright2020JS} allows describing the desired structure of a JSON file in terms of recursive rules, accounting for the fact that internal elements are either object or array nodes. For the former, each outgoing edge has a different, mandatory label, among an optionally specified list of possible labels, and children are unordered and can be subject to specific rules. For the latter, incoming edges are unlabeled, children are ordered, and one can specify a range for their number, as well as specific rules, for all or some of them. Additionally, JSON Schema provides syntactical mechanisms for specifying boolean combinations of rules and, thus, for taking the union, intersection, and complement of schemas.

\paragraph{Existing graph technologies}

openCypher Schema \cite{BonifatiFGHOV19} is a schema DDL for property graphs, whose main features are as follows. First, the language enables one to specify labels and mandatory property, thus strictly typing graph objects. Second, a schema validation mechanism is proposed, allowing to construct not only instances, but also schemas, as property graphs, thus facilitating introspection. Third, the formalism supports defining property keys. Additionally, graph rewriting rules facilitate update propagation between the instance and the schema, in a way that preserves consistency.

While not a graph database technology, in the narrow sense of the word, GraphQL~\cite{GraphQL2018,Hartig2018semantics} is based on a graph data model and schema formalism (SDL), consisting of a directed, edge-labeled multigraph. Its nodes are JSON-style objects, which contain a collection of fields, each with their own type and with values from back-end data stores (obtained using resolver functions). Its edges are specified by defining object fields, whose types are other object fields. Each object field has a mandatory name and type, as well as zero or more named arguments and directives (optional or required). An argument allows users to send data that can affect the outcome of GraphQL operations. When an argument is optional, it is possible to define a default value. A directive is an additional configuration that can extend each field with annotations. By default, every field in GraphQL is nullable, but users can change this using a non-null type modifier. GraphQL also supports interface and union types. 
%The former is an abstract type that holds a set of fields that a type must include to implement the interface. The latter provides an interface type, but it does not specify any common fields between the types. 
%GraphQL also proposes a simple DSL called Schema Definition Language (SDL) for defining schemas.
%It used to implement Web-based, client-driven APIs, facilitating the specification of a common abstraction layer between the client and the server. 

SQL/PGQ \cite{ISO9075,DeutschFGHLLLMM22} comprises the novel Part 16 of the SQL standard. This allows defining graph view schemas from SQL tables, as well as querying such views through a graph pattern matching mechanism that resembles that of Cypher, PGQL, and G-CORE.

AgensGraph \cite{AgensGDB} is a multi-model database based on PostgresQL. It supports the property graph data model, alongside the relational one and JSON documents, as well as uniform querying through both the SQL and openCypher languages.

ArangoDB \cite{arango:website} is a multi-model database system, in which data can be stored as key or value pairs, documents or graphs and uniformly queried using the AQL language. While ArangoDB is considered to be essentially schema-less, one can enforce structure at the document and collection levels using JSON Schema.

DataStax (DSG) \cite{datastax:website} is a real-time distributed graph database, which is tightly integrated with Apache Cassandra. The system's underlying model is that of a property graph and its query language leverages Apache TinkerPop's Gremlin functional language. DataStax's schema language allows one to define node and edge labels, as well as property keys and indexes.

JanusGraph \cite{JanusDB} is a scalable, distributed database system. It provides support for the property graph model, as exposed by Apache TinkerPop, and for querying it using the Gremlin graph traversal language. Graph schemas can be defined either explicitly, by specifying labels and properties for nodes and edges, or implicitly, through its \texttt{DefaultSchemaMaker}. This infers types that are natively supported by the system and automatically assigns single cardinality to property keys and multiple cardinality to edge labels.

Nebula Graph \cite{NebulaDB} is a distributed native graph database, whose data model is a directed property graph. The system is schema-full and also recommends limiting schema modifications (in particular at the level of node/edge properties), in accordance with its “strong-Schema” paradigm. It supports both openCypher and nGQL, a Nebula native query language.

Neo4j \cite{Neo4jDB} is a graph database that leverages the property graph model and its native Cypher query language. While  considered to be a schema-free system, Neo4j allows users to enforce the following constraints: unique node property, node and relationship property existence, as well as node key constraints. It also has a mechanism for automatically inferring the schema of a graph instance that, itself, is seen as a property graph that can be queried.
% Miller, Justin J. "Graph database applications and concepts with Neo4j." Proceedings of the southern association for information systems conference, Atlanta, GA, USA. Vol. 2324. No. 36. 2013.
% or/and
% Vukotic, Aleksa, et al. Neo4j in action. Vol. 22. Shelter Island: Manning, 2015.

Oracle/PGQL \cite{OracleSGDB,pgql} leverages a SQL-like query language for property graphs. Note that we focus only on its graph data model. Its DDL contains a \texttt{CREATE PROPERTY GRAPH} statement for building a graph from edge and node tables and storing it as a schema. Keys in node and edge tables uniquely identify these objects in the graph. 
% van Rest, Oskar, et al. "PGQL: a property graph query language." Proceedings of the Fourth International Workshop on Graph Data Management Experiences and Systems. 2016.

% Tesoriero, Claudio. Getting started with OrientDB. Birmingham, England: Packt Publishing, 2013.
OrientDB/SQL \cite{OrientDB} is a multi-model database whose engine was built to natively support the property graph, document, key/value and object models. The system can handle schema-less, schema-full, and schema-mixed modes, depending on how classes, i.e., node/edge labels, can be defined. In the first case, classes can either have no properties or only optional ones); in the second case, classes only have mandatory properties. In the third case, classes can have both mandatory and optional fields and, moreover, users can only set constraints for certain fields and add custom fields to records.

Sparksee \cite{SparkseeDB} is a graph database whose data model is a directed, label, attributed multigraph. It is a schema-full system, as types are mandatory, in order to create new graph objects, each of which has a unique and immutable OID. In terms of integrity restrictions, objects are only allowed one label, the only multi-valued attributes are \texttt{Array} ones, and attribute value uniqueness can be specified.

TigerGraph/GSQL \cite{TigerGraphDB,Deutsch19} is a graph database system in which users are required to define a fixed schema at the object level, i.e., node and edge types. The particularities of its GSQL schema definition are as follows. First, each edge type has a default primary key and an optional discriminator. This is a set of attributes that enables distinguishing between edges that share the same pair of source and target node instances. Even though, by default, the primary keys of the source and target nodes are used to uniquely identify edge instances, discriminators help to further differentiate these, when multiple ones link the same node pair. Second, edges can have reverse counterparts that share their schema and data, albeit having a different direction and name. Third, GSQL labels are semantic tags that can be attached to any group of graph elements. 
%Finally, types can have inheritance.
% Deutsch, Alin, et al. "Tigergraph: A native MPP graph database." arXiv preprint arXiv:1901.08248 (2019).

TypeDB/TypeQL \cite{TypeDB} is a strongly-typed database, whose rich type system fully implements the Entity-Relationship model, thus providing a concept-level schema, and whose underlying data model is that of a hypergraph. Moreover, its TypeQL native query language allows users to extract information from the graph data and its schema. It also allows reasoning about the data through rules that essentially correspond to Horn Clauses.
% You may consider cite it below, but it must be clarified that Grakn has changed its name to TypeDB
% Messina, Antonio, et al. "BioGrakn: A knowledge graph-based semantic database for biomedical sciences." Conference on Complex, Intelligent, and Software Intensive Systems. Springer, Cham, 2017.

%\newpage
